# Supplementary material for: AgentStore: Scalable Integration of Heterogeneous Agents As Specialized Generalist Computer Assistant
Source: arXiv:2410.18603 source file (2024-10-24)
Supplement: Supplementary file 1 [file appendix.tex]

\appendix
\input{app_osworld}
% You may include other additional sections here.
